# Supplementary material for: Block-STM: Scaling Blockchain Execution by Turning Ordering Curse to a Performance Blessing
Source: arXiv:2203.06871 source file (2022-08-25)
Supplement: Supplementary file 1 [file appendix.tex]

\section{Pseudocode}
\label{app:code}
In this section, we present the deferred pseudocode of 
the threshold logic in~\algorithmref{alg:parexec},
the \module{MVMemory} module in~\algorithmref{alg:data},
the \module{VM} execution in~\algorithmref{alg:vm},
the \module{Scheduler} module in~\algorithmref{alg:schvar} and~\algorithmref{alg:schdep}.

\input{alg-spawn}
\input{alg-memory}
\input{alg-vm}
\input{alg-scheduler}
\input{alg-execution}
\input{alg-validation}

% \section{More Evaluations}
\section{Anonymous Github Repositories}
\label{app:github}
Here we provide the links of the anonymous github repositories for our benchmarks of
\emph{Diem} p2p transactions
~\footnote{\url{https://anonymous.4open.science/r/Block-STM-EED6/README.md}},
\emph{Aptos} p2p transactions
~\footnote{\url{https://anonymous.4open.science/r/Block-STM-FF49/README.md}},
and our implementations of a variant of \textsc{Bohm}
\footnote{\url{https://anonymous.4open.science/r/Block-STM-FD0F/README.md}}
as well as LiTM
\footnote{\url{https://anonymous.4open.science/r/Block-STM-3CF6/README.md}} 
both in Rust in the Diem Blockchain.

\section{Aptos Evaluations}
\label{app:ev-aptos}
This section presents more evaluation results on Aptos p2p transactions (\figureref{fig:all-aptos}, \figureref{fig:bstm-high-aptos}, \figureref{fig:tps-aptos}), as previously described in \sectionref{sec:ev}.

\begin{figure*}[t]
\begin{minipage}[b]{0.45\linewidth}
    \centering
    \pgfplotsset{footnotesize,height=4.5cm, width=\linewidth}
    \begin{tikzpicture}
    \begin{axis}[
        scaled y ticks=base 10:-3,
        legend columns=4,
        % legend pos=north west,
        % legend pos=outer north,
        legend style={font=\footnotesize, at={(0.6,1.5)},anchor=north west},
        xlabel={Number of threads},
        ylabel= {Throughput},
        grid=major,
        xtick={4, 8, 16, 24, 32},
        ymin=0,
        ]
        %
        % \addplot [line width=0.25mm, color=magenta, mark=triangle] table [x=threads, y=bstm2,  col sep=comma] {plots/batch-1k};
        % %
        % \addplot [line width=0.25mm, color=red, mark=triangle] table [x=threads, y=bstm10,  col sep=comma] {plots/batch-1k};
        % %
        % \addplot [line width=0.25mm, color=cyan, mark=triangle] table [x=threads, y=bstm100,  col sep=comma] {plots/batch-1k};
        %
        \addplot [line width=0.25mm, color=blue, mark=triangle] table [x=threads, y=bstm1k,  col sep=comma] {plots/aptos-batch-1k};
        \addplot [line width=0.25mm, color=red, mark=triangle] table [x=threads, y=bstm10k,  col sep=comma] {plots/aptos-batch-1k};
        %
        % \addplot [line width=0.25mm, color=blue, mark=diamond] table [x=threads, y=litm1k,  col sep=comma] {plots/simple-batch-1k};
        % %
        % \addplot [line width=0.25mm, color=red, mark=diamond] table [x=threads, y=litm10k,  col sep=comma] {plots/simple-batch-1k};
        %
        % \addplot [line width=0.25mm, color=blue, mark=*] table [x=threads, y=bohm1kexe,  col sep=comma] {plots/simple-batch-1k-bohm};
        % %
        % \addplot [line width=0.25mm, color=red, mark=*] table [x=threads, y=bohm10kexe,  col sep=comma] {plots/simple-batch-1k-bohm};
        %
        \addplot [line width=0.25mm, black, mark=square] [error bars/.cd, y explicit,y dir=both,] table [x=threads, y=seq,  col sep=comma] {plots/aptos-batch-1k};
        %
        %
        % \addlegendentry{BSTM, 2 acc}
        % \addlegendentry{BSTM, 10 acc}
        % \addlegendentry{BSTM, 100 acc}
        \addlegendentry{BSTM, $10^3$ acc}
        \addlegendentry{BSTM, $10^4$ acc}
        % \addlegendentry{LiTM, $10^3$ acc}
        % \addlegendentry{LiTM, $10^4$ acc}
        % \addlegendentry{\textsc{Bohm}, $10^3$ acc}
        % \addlegendentry{\textsc{Bohm}, $10^4$ acc}
        \addlegendentry{Sequential}
    \end{axis}
    \end{tikzpicture}
\end{minipage}
\hspace{4ex}
\begin{minipage}[b]{0.45\linewidth}
    \centering
    \pgfplotsset{footnotesize,height=4.5cm, width=\linewidth}
    \begin{tikzpicture}
    \begin{axis}[
        scaled y ticks=base 10:-3,
        % legend pos=north west,
        % legend pos=outer north,
        xlabel={Number of threads},
        ylabel= {Throughput},
        grid=major,
        xtick={4, 8, 16, 24, 32},
        ymin=0,
        ]
        %
        % \addplot [line width=0.25mm, color=magenta, mark=triangle] table [x=threads, y=bstm2,  col sep=comma] {plots/batch-1k};
        % %
        % \addplot [line width=0.25mm, color=red, mark=triangle] table [x=threads, y=bstm10,  col sep=comma] {plots/batch-1k};
        % %
        % \addplot [line width=0.25mm, color=cyan, mark=triangle] table [x=threads, y=bstm100,  col sep=comma] {plots/batch-1k};
        %
        \addplot [line width=0.25mm, color=blue, mark=triangle] table [x=threads, y=bstm1k,  col sep=comma] {plots/aptos-batch-10k};
        \addplot [line width=0.25mm, color=red, mark=triangle] table [x=threads, y=bstm10k,  col sep=comma] {plots/aptos-batch-10k};
        %
        % \addplot [line width=0.25mm, color=blue, mark=diamond] table [x=threads, y=litm1k,  col sep=comma] {plots/simple-batch-10k};
        % %
        % \addplot [line width=0.25mm, color=red, mark=diamond] table [x=threads, y=litm10k,  col sep=comma] {plots/simple-batch-10k};
        % %
        % \addplot [line width=0.25mm, color=blue, mark=*] table [x=threads, y=bohm1kexe,  col sep=comma] {plots/simple-batch-10k-bohm};
        % %
        % \addplot [line width=0.25mm, color=red, mark=*] table [x=threads, y=bohm10kexe,  col sep=comma] {plots/simple-batch-10k-bohm};
        %
        \addplot [line width=0.25mm, black, mark=square] [error bars/.cd, y explicit,y dir=both,] table [x=threads, y=seq,  col sep=comma] {plots/aptos-batch-10k};
    \end{axis}
    \end{tikzpicture}
\end{minipage}
\caption{Comparison of BSTM and Sequential execution for block size $10^3$ (left) and $10^4$ (right). Aptos p2p transactions.}
\label{fig:all-aptos}
\end{figure*}

\begin{figure}[H]
    \centering
    \pgfplotsset{footnotesize,height=4.5cm, width=\linewidth}
    \begin{tikzpicture}
    \begin{axis}[
        scaled y ticks=base 10:-3,
        legend columns=2,
        % legend pos=north west,
        % legend pos=outer north,
        legend style={font=\footnotesize, at={(0.0,1.8)},anchor=north west,legend columns=2},
        xlabel={Number of threads},
        ylabel= {Throughput},
        grid=major,
        xtick={4, 8, 16, 24, 32},
        ymin = 0,
        ]
        \addplot [line width=0.25mm, color=magenta, mark=triangle] table [x=threads, y=bstm2,  col sep=comma] {plots/aptos-batch-1k};
        \addplot [line width=0.25mm, color=blue, mark=triangle] table [x=threads, y=bstm10,  col sep=comma] {plots/aptos-batch-1k};
        \addplot [line width=0.25mm, color=cyan, mark=triangle] table [x=threads, y=bstm100,  col sep=comma] {plots/aptos-batch-1k};
        \addplot [line width=0.25mm, color=yellow, mark=diamond] table [x=threads, y=bstm2,  col sep=comma] {plots/aptos-batch-10k};
        \addplot [line width=0.25mm, color=green, mark=diamond] table [x=threads, y=bstm10,  col sep=comma] {plots/aptos-batch-10k};
        \addplot [line width=0.25mm, color=red, mark=diamond] table [x=threads, y=bstm100,  col sep=comma] {plots/aptos-batch-10k};
        \addplot [line width=0.25mm, black, mark=square] [error bars/.cd, y explicit,y dir=both,] table [x=threads, y=seq,  col sep=comma] {plots/aptos-batch-1k};
        \addlegendentry{BSTM, 2 acc, $10^3$ bch}
        \addlegendentry{BSTM, 10 acc, $10^3$ bch}
        \addlegendentry{BSTM, 100 acc, $10^3$ bch}
        \addlegendentry{BSTM, 2 acc, $10^4$ bch}
        \addlegendentry{BSTM, 10 acc, $10^4$ bch}
        \addlegendentry{BSTM, 100 acc, $10^4$ bch}
        \addlegendentry{Sequential}
    \end{axis}
    \end{tikzpicture}
    \caption{Comparison of BSTM and sequential execution for block size $10^3$ and $10^4$, account sizes 2, 10 and 100. Aptos p2p transactions.}
    \label{fig:bstm-high-aptos}
\end{figure}

\begin{figure}[H]
    \centering
    \pgfplotsset{footnotesize,height=4.5cm, width=\linewidth}
    \begin{tikzpicture}
    \begin{axis}[
        scaled ticks=base 10:-3,
        legend columns=2,
        % legend pos=north west,
        % legend pos=outer north,
        legend style={font=\small, at={(0,1.5)},anchor=north west,legend columns=2},
        xlabel={Block size},
        ylabel= {Throughput},
        grid=major,
        xtick={1000, 5000, 10000, 20000, 50000},
        ]
        \addplot [line width=0.25mm, color=magenta, mark=triangle] table [x=batches, y=bstm-16-1k,  col sep=comma] {plots/aptos-batches};
        \addplot [line width=0.25mm, color=blue, mark=triangle] table [x=batches, y=bstm-16-10k,  col sep=comma] {plots/aptos-batches};
        \addplot [line width=0.25mm, color=cyan, mark=*] table [x=batches, y=bstm-32-1k,  col sep=comma] {plots/aptos-batches};
        \addplot [line width=0.25mm, color=purple, mark=*] table [x=batches, y=bstm-32-10k,  col sep=comma] {plots/aptos-batches};
        \addlegendentry{16 threads, $10^3$ acc}
        \addlegendentry{16 threads, $10^4$ acc}
        \addlegendentry{32 threads, $10^3$ acc}
        \addlegendentry{32 threads, $10^4$ acc}
    \end{axis}
    \end{tikzpicture}
    \caption{Throughput of BSTM for various block sizes. Aptos p2p transactions.}
    \label{fig:tps-aptos}
\end{figure}
